# Supplementary material for: Chiral and helical $p$-wave superconductivity in doped bilayer BiH
Source: arXiv:1809.06103 source file (2018-09-17)
Supplement: Supplementary file 1 [file Supplemental.pdf]

# Supplemental Materials for "Chiral and helical $p$-wave superconductivity in doped bilayer BiH"

Lin Yang,[1] Wan-Sheng Wang,[2] Da Wang,[1] and Qiang-Hua Wang[1,3,*]

[1]*National Laboratory of Solid State Microstructures & School of Physics, Nanjing University, Nanjing, 210093, China*
[2]*Department of Physics, Ningbo University, Ningbo 315211, China*
[3]*Collaborative Innovation Center of Advanced Microstructures, Nanjing University, Nanjing 210093, China*

Here we describe the technical details of SM-FRG and the FRG-derived mean field theory.

In Sec.S1-S3 we describe technical details in SM-FRG. In simple terms, SM-FRG is a realization of FRG, originally proposed by Wetterich,[1] in terms of scattering of truncated fermion bilinears that are sufficient to capture the potentially singular scattering modes in correlated electron systems.[2–11] We also describe in Sec.S4 the FRG-derived mean field theory for the ordered state below $T_c$.

## S1. FRG FLOW EQUATION

The idea of FRG is to obtain the 1PI interaction vertices $\Gamma_{1234}$, as in $H_\Gamma = \sum_{1234} \psi_1^\dagger \psi_2^\dagger \Gamma_{1234} \psi_3 \psi_4/(2!)^2$, for quasi-particles above a running infrared energy cut off $\Lambda$ (which we take as the lower limit of the continuous Matsubara frequency). The numerical subscript $1 = (\mathbf{k}, a, s)$ labels (momentum, orbital, spin), and momentum conservation is assumed implicitly. (We include the sublattice into the orbital for brevity.) Equivalently, $\Gamma_{1234}$ may be taken as the effective interactions on quasiparticles below the scale $\Lambda$, in the spirit of pseudopotential. Starting from $\Lambda = \infty$ where $H_\Gamma$ is specified by the bare interaction $H_I$, the contribution to the flow (toward decreasing $\Lambda$) of the vertex, $\partial\Gamma_{1234}/\partial\Lambda$, is illustrated in the main text, and is reproduced here for convenience in Fig.S1.

Before proceeding, we notice that for a system with featureless Fermi surface(s), standard RG dimension-counting reveals that all four-point interactions are marginal. This means higher-order vertices and the frequency dependence in the 4-point vertex $\Gamma_{1234}$ are irrelevant and can be dropped, as long as instabilities occur at low energy scales (to justify the RG argument). In this approximation, the single-particle self-energy correction in during the FRG flow is frequency independent and can be absorbed in the normal state Hamiltonian. In fact, this type of approximation is also valid in two-dimensional models even if there is a vHS right at the Fermi level. In this case the fermion dispersion is hyperbolic near the vHS, $\epsilon_{\mathbf{q}} \sim a_1 q_x^2 - a_2 q_y^2$, where $\mathbf{q}$ is the momentum deviation from the vHS, and $a_{1,2}$ are model dependent coefficients. Then the frequency $\omega$ scales as $q^2$ (or the dynamical exponent is $z = 2$), and consequently the fermion field $\psi$ scales as $q^{-3}$. The $n$-point vertex function scales as $q^{3n-4(n-1)} = q^{4-n}$, which is therefore also marginal for $n = 4$ and irrelevant for $n > 4$. We will therefore concentrate on the flow of $\Gamma_{1234}$ only.

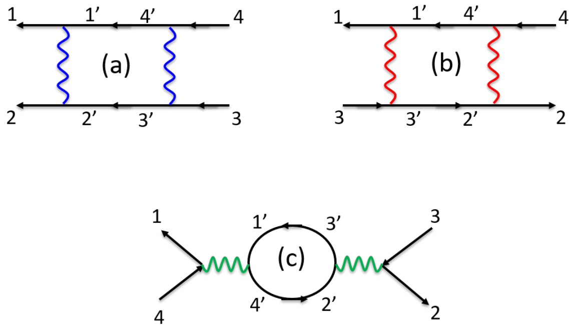


FIG. S1: One-loop diagrams contributing to $\partial\Gamma_{1234}/\partial\Lambda$, quadratic in $\Gamma$ itself (wavy lines, fully antisymmetrized with respect to incoming or outgoing fermions, labelled by the numerical indices). The color of the wavy line signifies scattering of fermion bilinears in the (a) pairing, (b) crossing and (c) direct channel.

It turns out to be useful to view $\Gamma$ as scattering matrices for fermion bilinears,

$$\Gamma_{1234} = P_{12,43} = C_{13,42} = D_{14,32}, \tag{S1}$$

where $P$ is the matrix in the pp channel, and $C$ and $D$ in the ph channel. Then the RG flow equation, shown schematically in Fig.S1, can be written compactly as

$$\begin{aligned}\frac{\partial\Gamma_{1234}}{\partial\Lambda} = & -\frac{1}{2}[P\chi'_{pp}P]_{12,43} + [C\chi'_{ph}C]_{13,42} \\ & -[D\chi'_{ph}D]_{14,32},\end{aligned} \tag{S2}$$

where the products within the square brackets are understood as convolution in the bilinear labels, see Fig.S1, and $\chi'_{pp/ph}$ are differential susceptibilities, as matrices in the bilinear basis,

$$\begin{aligned}[\chi'_{pp}]_{12,34} &= \frac{\partial}{\partial\Lambda}\int_{|\omega|\geq\Lambda}\frac{d\omega}{2\pi}G_{13}(i\omega)G_{24}(-i\omega), \\ [\chi'_{ph}]_{12,34} &= -\frac{\partial}{\partial\Lambda}\int_{|\omega|\geq\Lambda}\frac{d\omega}{2\pi}G_{13}(i\omega)G_{42}(i\omega),\end{aligned} \tag{S3}$$

where $G_{12}(i\omega_n) = -\langle\psi_1(i\omega_n)\bar{\psi}_2(i\omega_n)\rangle$ is the normal state Matsubara Green's function. In actual calculations, the loop integration in Eq.S2 is performed in momentum space.

## S2. SINGULAR SCATTERING MODES

As $\Gamma$ flows with decreasing scale $\Lambda$, a diverging or singular eigenmode of a scattering matrix at a scale $\Lambda_c$ signals an instability of the normal state at the transition temperature $T_c \sim \Lambda_c$, and also tells the internal structure of the emerging order. To basic idea is most easily explained by ignoring the orbital and spin labels for the moment. Let us consider fermion bilinears limited to a set of relative displacement $\mathbf{r}$, say $\mathbf{r} \in (\mathbf{r}_m, m = 1, \cdots)$. We first rewrite the effective interaction $H_\Gamma$ on quasiparticles as, up to an unimportant global factor,

$$\begin{aligned} H_\Gamma &\sim \bar{\psi}_{\mathbf{R}_0}\bar{\psi}_{\mathbf{R}_0+\mathbf{r}_m} P_{mn}(\mathbf{R})\psi_{\mathbf{R}+\mathbf{R}_0+\mathbf{r}_n}\psi_{\mathbf{R}+\mathbf{R}_0} \\ &= \bar{\psi}_{\mathbf{k}+\mathbf{q}}\bar{\psi}_{-\mathbf{k}} f_m(\mathbf{k}) P_{mn}(\mathbf{q}) f_n^*(\mathbf{k}')\psi_{-\mathbf{k}'}\psi_{\mathbf{k}'+\mathbf{q}}. \end{aligned} \quad \text{(S4)}$$

Henceforth, summation over repeated indices are implied for brevity, unless specified otherwise. The first (second) line is in the real (momentum) space, $P_{mn}(\mathbf{R}) \equiv P_{(0,\mathbf{r}_m),(\mathbf{R},\mathbf{R}+\mathbf{r}_n)}$, and $f_l(\mathbf{k}) = e^{i\mathbf{k}\cdot\mathbf{r}_l}$ is a basic lattice harmonics, or form factor. The matrix $P(\mathbf{q})$ is hermitian and can be decomposed as, dropping $\mathbf{q}$ for brevity,

$$P_{mn} = \sum_\alpha \phi_m^\alpha S_\alpha \phi_n^{\alpha *}, \quad \text{(S5)}$$

where $\alpha$ labels the eigenstate $\phi^\alpha$ with eigenvalue $S_\alpha$. Suppose there is a most negative eigenvalue (MNE) $S$ associated with an eigenfunction $\phi$ at $\mathbf{q} = \mathbf{Q}$, we have

$$H_\Gamma \sim \bar{\psi}_{\mathbf{k}+\mathbf{Q}}\bar{\psi}_{-\mathbf{k}} f_m(\mathbf{k})\phi_m S \phi_n^* f_n^*(\mathbf{k}')\psi_{-\mathbf{k}'}\psi_{\mathbf{k}'+\mathbf{Q}} + \cdots \quad \text{(S6)}$$

The divergence of $S$ implies an emerging Cooper pairing at collective momentum $\mathbf{Q}$ with the pairing function

$$\phi(\mathbf{k}) = \sum_m \phi_m f_m(\mathbf{k}). \quad \text{(S7)}$$

By Cooper mechanism, the most favorable collective momentum is $\mathbf{Q} = 0$ for time-reversal-invariant systems. $\phi(\mathbf{k})$ forms an irreducible representation of the little group at $\mathbf{Q}$, and degeneracy exists if it belongs to a multiplet irreducible representation.

Similarly, we can rewrite $H_\Gamma$ in terms of $D$ as

$$\begin{aligned} H_\Gamma &\sim \bar{\psi}_{\mathbf{R}_0}\psi_{\mathbf{R}_0+\mathbf{r}_m} D_{mn}(\mathbf{R})\bar{\psi}_{\mathbf{R}_0+\mathbf{R}+\mathbf{r}_n}\psi_{\mathbf{R}_0+\mathbf{R}} \\ &= \bar{\psi}_{\mathbf{k}+\mathbf{q}}\psi_{\mathbf{k}} f_m(\mathbf{k}) D_{mn}(\mathbf{q}) f_n^*(\mathbf{k}')\bar{\psi}_{\mathbf{k}'}\psi_{\mathbf{k}'+\mathbf{q}} \\ &\sim \bar{\psi}_{\mathbf{k}+\mathbf{Q}}\psi_{\mathbf{k}} f_m(\mathbf{k})\phi_m S \phi_n^* f_n^*(\mathbf{k}')\bar{\psi}_{\mathbf{k}'}\psi_{\mathbf{k}'+\mathbf{Q}} + \cdots \end{aligned} \quad \text{(S8)}$$

where $D_{mn}(\mathbf{R}) = D_{(0,\mathbf{r}_m),(\mathbf{R},\mathbf{R}+\mathbf{r}_n)}$, and the dotted part is for subleading terms. In the last step we assume the matrix $D(\mathbf{q})$ has a MNE $S$ associated with the eigenfunction $\phi$ at momentum $\mathbf{q} = \mathbf{Q}$. The divergence of $S$ implies an emerging density-wave order in the ph channel, and the structure of order parameter is described again by the function $\phi(\mathbf{k}) = \sum_m \phi_m f_m(\mathbf{k})$, but now for the ph pair. If it is independent (dependent) of $\mathbf{k}$, it describes site-local (bond-centered) density-wave order. Coexistence of site-local and bond-centered density-wave can also be captured. Notice that $\mathbf{Q} = 0$ is not generally favorable in the ph channel (unless at a vHS), and for $\mathbf{Q} \neq 0$ there is degeneracy in $\mathbf{Q}$'s related by point group symmetry.

We now include the other internal degrees of freedom. To each $\mathbf{r}_m$ we associate a pair of orbitals $aa'$ and a pair of spins $ss'$. We can group the orbital and spin into a combined label $\mu = (a, s)$. The leading eigenfunction $\phi^{\mu\mu'}(\mathbf{k})$ now becomes a matrix, providing additional informations on pairing of orbitals and spins in the order parameter (applicable for both pp and ph channels), as discussed in the main text.

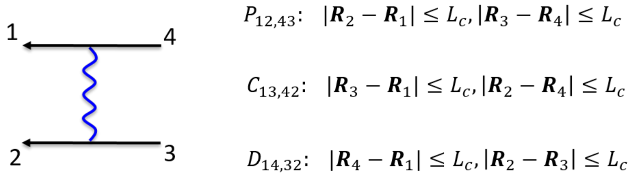


FIG. S2: Illustration of assignment of a 4-point vertex $\Gamma_{1234}$ into the three scattering channels according to the truncation length $L_c$. A vertex is an overlap if the assignment can be made in two or all of the three channels.

## S3. TRUNCATION OF FERMION BILINEARS

The flow equation in the form of Eq.S2 is still not useful if fermion bilinears with unlimited relative displacement $\mathbf{r}$ are all kept, the number of which diverges in the thermodynamic limit. We argue that only a finite set of $\mathbf{r}$'s are important in a potentially diverging (or singular) scattering mode, the underlying idea of SM-FRG. We observe that if only one out of $P$, $C$ and $D$ is retained in Eq.S2, the flow equation reduces to the ladder approximation for $P$ in the pp channel, and to the random phase approximation for $C$ (or $D \equiv -C$ because of full antisymmetrization) in the ph channel. One would be able to address instabilities in such channels separately. Although subject to serious biases, these approximations do help demonstrate how a generally marginal 4-point vertex could become relevant: by repeated and coherent scattering of fermion bilinears. When an eigen scattering mode becomes singular (or has a diverging eigenvalue), it signals an instability of the normal state, as we discussed above. Since in all known examples of ordered state, the order parameter is local or short-ranged, such as local $s$-wave pairing, $d$-wave pairing on bond, site-local density-waves, etc., it is perceivable that the most important fermion bilinears (in the respective scattering channel) that would enter a singular scattering mode are local or short-ranged. (This is not withstanding possible long-range correlations between fermion bilinears.) In fact, unless it is attractive already at the tree level, a scattering channel could become attractive and singular during RG only by

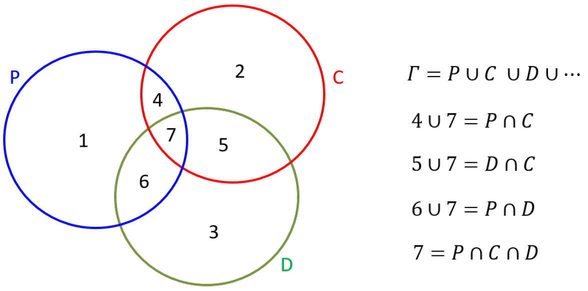


FIG. S3: The relation among truncated $P$, $C$, $D$ and the full vertex $\Gamma$ in terms of set theory. Without truncation, $P$, $C$ and $D$ are fully overlapped and are simply aliases of $\Gamma$. After truncation the overlaps are partial but sufficient for potentially singular scattering modes in pp and ph channels.

its overlap with the other channel, as is clear in the flow equation. If the overlap is strong and very nonlocal, the doner channel must have developed strong nonlocal correlations and hence may diverge even faster. Therefore, we can truncate the relative spatial range in the bilinears entering $P$, $C$ and $D$, say up to a length scale $L_c$. (The setback distance between fermion bilinears is unlimited.) Fig.S2 shows how in real space a 4-point vertex is ascribed to $P$, $C$ or $D$. A vertex is overlapped if it can be ascribed to two or all of the truncated scattering channels. In fact, limiting the fermion bilinears to site-local spin-density and $d$-wave pairing on first-neighbor bonds proved already successful for the Hubbard model describing cuprates.[12]

Without truncation, $P$, $C$ and $D$ are simply aliases of $\Gamma$. With truncation they capture only parts of $\Gamma$ which are most important according to the above arguments. The overlaps between them are shown schematically in Fig.S3. In SM-FRG, Eq.S2 is integrated step by step, and after each step, $P$, $C$ and $D$ are reassigned by $\Gamma$ according to Eq.S1 and Fig.S2. This scheme is asymptotically exact for parametrization of $\Gamma$ as $L_c$ is enlarged. A finite truncation makes the calculation feasible, and is sufficient to capture, on equal footing, general pp and ph order parameters defined on site and on short-ranged bonds. Notice that the loop integration is performed in momentum space, but the overlaps between the scattering matrices are handled most conveniently in real space, since overlaps are restricted by the truncation length in fermion bilinears, see Fig.S2.

In the SM-FRG calculations for the main text, we take $L_c$ to be the length of the second-neighbor bond. However, the leading scattering modes in the pp and ph channels are all dominated by onsite fermion bilinears, showing $L_c$ is sufficiently large in our case.

## S4. FRG-DERIVED MEAN FIELD THEORY

Finally, we discuss how to describe the ordered state below $T_c$, given the FRG-derived pairing function. This is necessary if the pairing function is degenerate and we need to know how they would recombine in the ordered state. What we need is a mean field theory as specified in the main text. The effective pair interaction used in Eq.10 (of the main text) can be regarded as the 2PI part of $S_{\rm pp}$ in FRG via

$$S_{\rm pp}^{-1} = V^{-1} + \chi, \tag{S9}$$

which holds when the pp and ph channels are essentially decoupled (as $\Lambda \to \Lambda_c$). Here $\chi$ is the pair susceptibility for a given pairing mode, and is contributed by quasiparticles above the scale $\Lambda$. With $V$ extracted this way, the mean field $T_c$ is just $\Lambda_c$. In practice we can simply tune the value of $V$ so that $T_c = \Lambda_c$. This can be taken as an FRG-derived mean field theory. For illustrative purpose, we also enlarged $V$ to get a larger pairing gap in Figs.5 and 6 of the main text.

* Electronic address: qhwang@nju.edu.cn


1 C. Wetterich, Phys. Lett. B. **301**, 90 (1993).
2 Q.-H. Wang, C. Platt, Y. Yang, C. Honerkamp, F. C. Zhang, W. Hanke, T. M. Rice, and R. Thomale, EPL **104**, 17013 (2013).
3 W.-S. Wang, Y.-Y. Xiang, Q.-H. Wang, F. Wang, F. Yang, and D.-H. Lee, Phys. Rev. B. **85**, 035414 (2012).
4 Y.-Y. Xiang, W.-S. Wang, Q.-H. Wang, and D.-H. Lee, Phys. Rev. B. **86**, 024523 (2012).
5 W.-S. Wang, Z.-Z. Li, Y.-Y. Xiang, and Q.-H. Wang, Phys. Rev. B. **87**, 115135 (2013).
6 Y.-Y. Xiang, F. Wang, D. Wang, Q.-H. Wang, and D.-H. Lee, Phys. Rev. B **86**, 134508 (2012).
7 Y.-Y. Xiang, Y. Yang, W.-S. Wang, Z.-Z. Li, and Q.-H. Wang, Phys. Rev. B **88**, 104516 (2013).
8 Y. Yang, W.-S. Wang, Y.-Y. Xiang, Z.-Z. Li, and Q.-H. Wang, Phys. Rev. B **88**, 094519 (2013).
9 W.-S. Wang, M. Gao, Y. Yang, Y.-Y. Xiang, and Q.-H. Wang, Phys. Rev. B **95**, 144507 (2017).
10 Y. Wang, J.-G. Liu, W.-S. Wang, and Q.-H. Wang, Phys. Rev. B. **97**, 174513 (2018).
11 Y.-C. Liu, W.-S. Wang, F.-C. Zhang, and Q.-H. Wang, Phys. Rev. B **97**, 224522 (2018).
12 C. Husemann and M. Salmhofer, Phys. Rev. B. **79**, 195125 (2009)
